# Supplementary material for: TuneAhead: Predicting Fine-tuning Performance Before Full Training Begins
Source: arXiv:2606.17660 source file (2026-06-16)
Supplement: Supplementary file 1 [file appen_generalization.tex]

%!TEX root = ../main.tex
\clearpage
\section{Cross-Model Generalization}
\label{app:generalization}

\paragraph{Motivation.}
A key question regarding our findings is whether the \sys framework is specific to the Qwen2-7B-Instruct model used in our main experiments, or if its principles generalize to other settings.
To address this, we conducted two additional sets of experiments to validate the robustness of our approach across a different model architecture (Llama) and a significantly smaller model scale (0.5B).

\paragraph{Experimental Setup.}
We created two new, independent meta-datasets.
\begin{description}[leftmargin=1.2em]
  \item[Different Architecture.] We used \texttt{Llama-3-8B-Instruct} as the base model and replicated our entire meta-dataset curation process, resulting in only 400 new fine-tuning runs.
  \item[Different Scale.] We used \texttt{Qwen2-0.5B-Instruct} as the base model and repeated the process again for only 450 runs.
\end{description}
For each of these new base models, we trained a separate \sys predictor from scratch using the exact same feature engineering and modeling methodology described in Sec.~\ref{sec:solution}.

\begin{table}[t]
  \centering
  \setlength{\tabcolsep}{6pt}
  \begin{tabular}{lrrrrrr}
    \toprule
    Base Model & \multicolumn{1}{c}{RMSE $\downarrow$} & \multicolumn{1}{c}{$R^2 \uparrow$} & \multicolumn{1}{c}{$r \uparrow$} & \multicolumn{1}{c}{Acc@1pp $\uparrow$} & \multicolumn{1}{c}{Acc@2pp $\uparrow$} & \multicolumn{1}{c}{Acc@3pp $\uparrow$} \\
    \midrule
    Llama-3-8B-Instruct   & 5.02 & 0.86 & 0.93 & 36.00 & 55.80 & 73.30\\
    Qwen2-0.5B   & 3.75  & 0.91  & 0.95 & 39.20  & 58.40 & 74.60  \\
    \bottomrule
  \end{tabular}
  \caption{Cross-model generalization results for \sys on two new meta-datasets. Across both a different architecture (Llama-3-8B) and a much smaller scale (Qwen2-0.5B), the framework maintains low RMSE and high Acc@$k$pp, indicating strong generalization beyond the Qwen2-7B-Instuct setting.}
  \label{tab:d1-results}
\end{table}

\paragraph{Results.}
The performance of \sys on these new meta-datasets is summarized in Table~\ref{tab:d1-results}.
We observe that \sys consistently maintains low RMSE and reasonably high Acc@$k$pp across both settings. 
In particular, even on the small-scale Qwen2-0.5B meta-dataset, the framework still achieves $R^2=0.69$ and 
Acc@3pp of 63.0, showing that meaningful predictive signal is captured despite the limited sample size. 
These results support the robustness and cross-model generalization of \sys beyond the model scale and architecture setting.
